# Supplementary material for: Enhanced Light-Matter Interaction in Graphene/h-BN van der Waals Heterostructures
Source: arXiv:1703.06035 source file (2017-03-17)
Supplement: Supplementary file 1 [file supp_info_REVISED.pdf]

# SUPPORTING INFORMATION

# Enhancing Light-Matter Interaction in Graphene/h-BN van der Waals heterostructures

Wahib Aggoune,[†,‡] Caterina Cocchi,[*,†,¶] Dmitrii Nabok,[†,¶] Karim Rezouali,[‡] Mohamed Akli Belkhir,[‡] and Claudia Draxl[†,¶]

†*Institut für Physik and IRIS Adlershof, Humboldt-Universität zu Berlin, 12489 Berlin, Germany*

‡*Laboratoire de Physique Théorique, Faculté des Sciences Exactes, Université de Bejaia, 06000 Bejaia, Algeria*

¶*European Theoretical Spectroscopic Facility (ETSF)*

E-mail: caterina.cocchi@physik.hu-berlin.de

# Graphene/h-BN Periodic Heterostructures: Structural and Electronic Properties

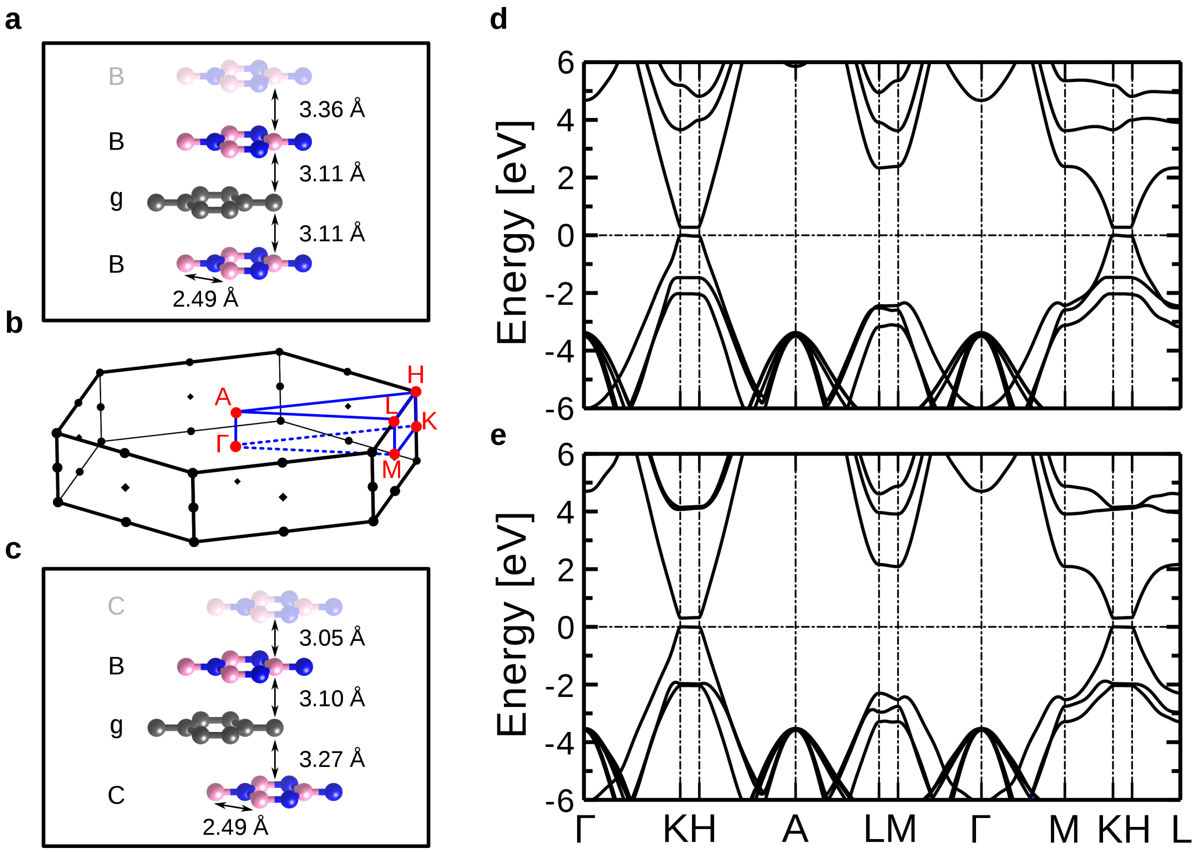


Figure S1: Stacking arrangements of the two heterostructures considered in this work, with B-g-B and B-g-C stacking arrangements (a and c, respectively). The corresponding Brillouin zone (BZ) is also shown (b), with the high-symmetry points marked in red. Quasi-particle band structures of (d) B-g-B and (e) B-g-C heterostructures along the path in the BZ highlighted in (b), with the valence-band maximum set to zero.

The unit cells of the graphene/h-BN heterostructures considered in this work contain 6 atoms, and have in-plane lattice parameter $a$=2.49 Å. In the B-g-B stacking arrangement (Fig. S1a), $c$=9.58 Å. In this configuration, the graphene layer is separated by 3.11 Å from the h-BN ones, while two neighboring h-BN sheets are at a vertical distance of 3.36 Å. In the B-g-C heterostructure $c$=9.42 Å. In this system, the distance between graphene and the h-BN layers in stacking position B and C is 3.10 Å and 3.27 Å, respectively. In this stacking sequence, the distance between two neighboring boron nitride sheets is 3.05 Å.

In Figs. S1d-e we show the full band structure of the graphene/h-BN periodic heterostructures along the **k**-point path highlighted in Fig. S1b. These plots are obtained by Wannier interpolation starting from a calculation using a 12×12×4 **k**-mesh. The systems exhibit a quasi-particle gap of 250 meV (B-g-B) and 260 meV (B-g-C) between the graphene-like highest-occupied and lowest-unoccupied bands along the K-H path. Along the L-M path the separation between the N-like valence-band maximum (VBM) and the C-like conduction-band minimum (CBM) is significantly larger, being 4.7 eV in B-g-B and 4.5 eV in B-g-C.

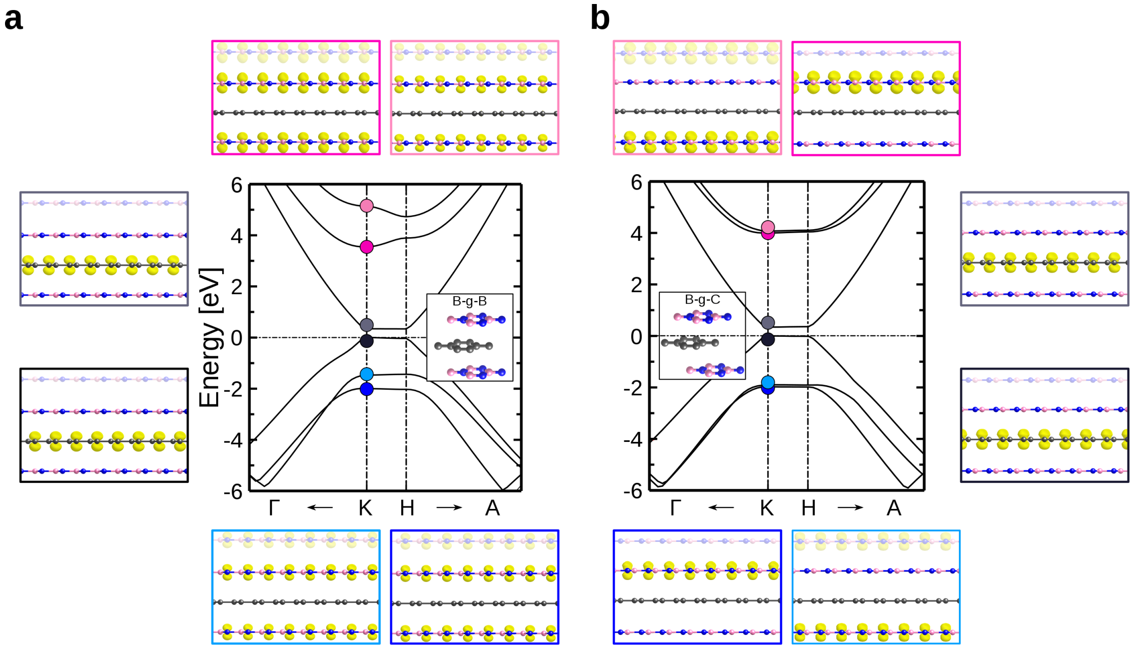


Figure S2: Quasi-particle band structure in the vicinity of the K-H path and electron probability density at K of the three highest occupied and the three lowest unoccupied Kohn-Sham states of the B-g-B (a) and the B-g-C (b) heterostructures. The three layers included in the unit cell are shown in the foreground, while periodic images are shaded.

In Fig. S2 we show the spatial extension of the electron density associated with the three lowest occupied and unoccupied Kohn-Sham (KS) states at the high-symmetry point K. Regardless of the stacking order, the VBM and the CBM are purely graphene-like $\pi$ and $\pi^*$ states, respectively, exhibiting their typical delocalized distribution on the two inequivalent carbon atoms in the unit cell. In the B-g-B system, VBM-1 and VBM-2 are extended N

states, while CBM+1 and CBM+2 show a boron-like character. In both cases, the electron distribution is uniformly spread over both h-BN layers included in the unit cell. This is a direct consequence of the equivalent arrangement of the h-BN sheets with respect to each other. On the other hand, in the B-g-C heterostructure VBM-1 and VBM-2 as well as CBM+1 and CBM+2 are almost degenerate at K and their corresponding electron density is distributed on one inequivalent h-BN layer.

## Graphene/h-BN Heterostructures: Optical Properties

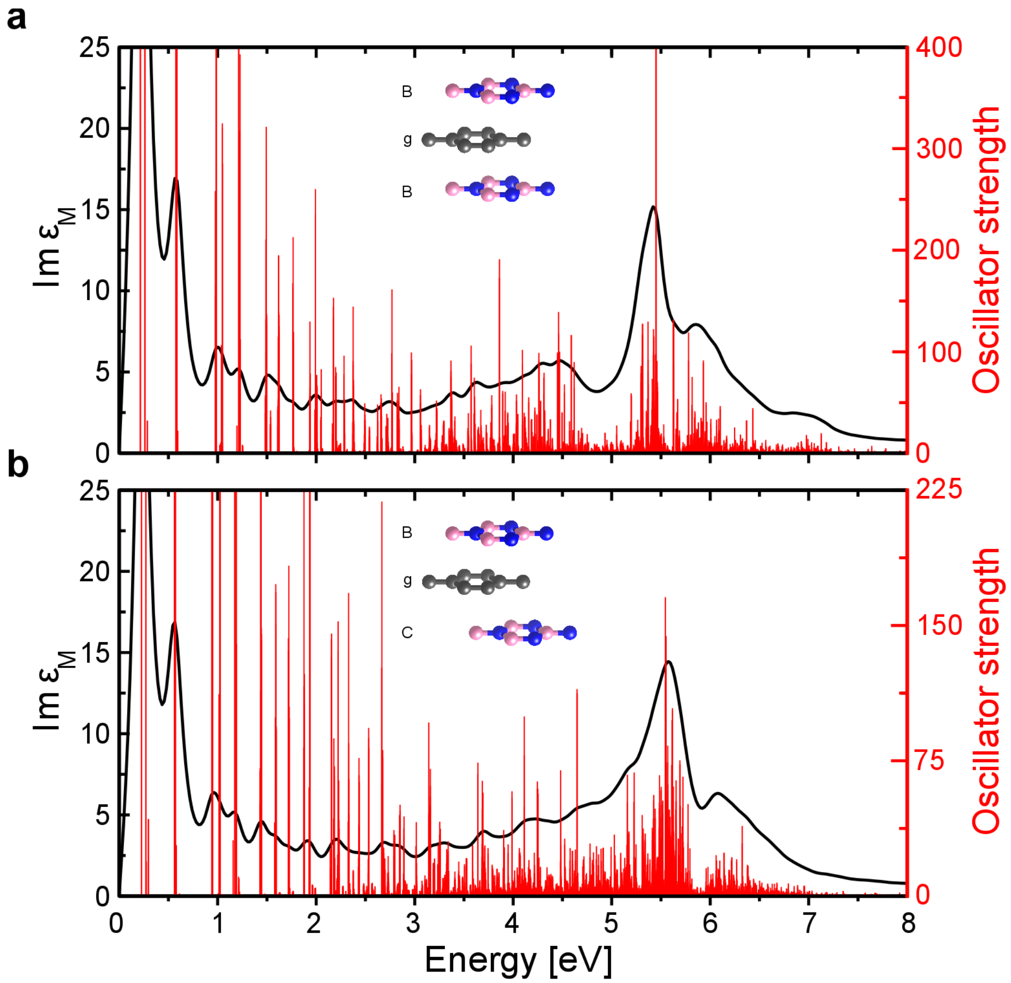


Figure S3: In-plane component of the imaginary part of the macroscopic dielectric function (black solid line) and oscillator strength of the corresponding solution of the BSE (red bars) of B-g-B (a) and B-g-C (b) heterostructures.

In Fig. S3 we show the in-plane component of the imaginary part of the macroscopic dielectric function and the oscillator strength of the corresponding solutions of the Bethe-Salpeter equation (BSE) for the B-g-B and B-g-C stacking arrangements. In main text (Figs. 1a and 2a) we highlight only selected excitations with specific character, not necessarily corresponding to the most intense ones. Specifically, in the visible region, most of the spectral intensity comes from excitations formed by a mixture of transitions between the three highest-occupied bands to the graphene-like CBM. As discussed in main body of the article, many excitations are double-degenerate for symmetry reasons. As such, the correlated probability density associated to the electron, with the hole being fixed, is a linear combination of the single contribution of the degenerate BSE solutions. Significant examples, corresponding to each type of excitation discussed in the main text is shown in Fig. S4. It is worth noting, in particular, that the correlated electron distribution of the intralayer exciton in the h-BN layer (Fig. S4c) is consistent with the results reported in Ref. 1.

# Exciton Analysis in k-Space

In this section, we provide an additional analysis of the excitations highlighted in Figs. 1 and 2 in the main text. Specifically we consider here the **k**-resolved contributions of individual quasi-particle bands to the electron-hole pairs. To do so, we introduce the *weight* of each transition between valence and conduction states at a given **k**-point, defined as:

$$w^{\lambda}_{v\mathbf{k}} = \sum_{c} |A^{\lambda}_{vc\mathbf{k}}|^2, \;\; w^{\lambda}_{c\mathbf{k}} = \sum_{v} |A^{\lambda}_{vc\mathbf{k}}|^2. \tag{1}$$

In Figs. S5 and S6 these quantities are plotted as colored circles, whose size is representative of the **k**-resolved band contributions, independently of the oscillator strength of the corresponding excitation.

In Fig. S5 we show the most relevant contributions to the excitations in the spectra of graphene/h-BN heterostructures with B-g-B stacking sequence. Excitations are labeled

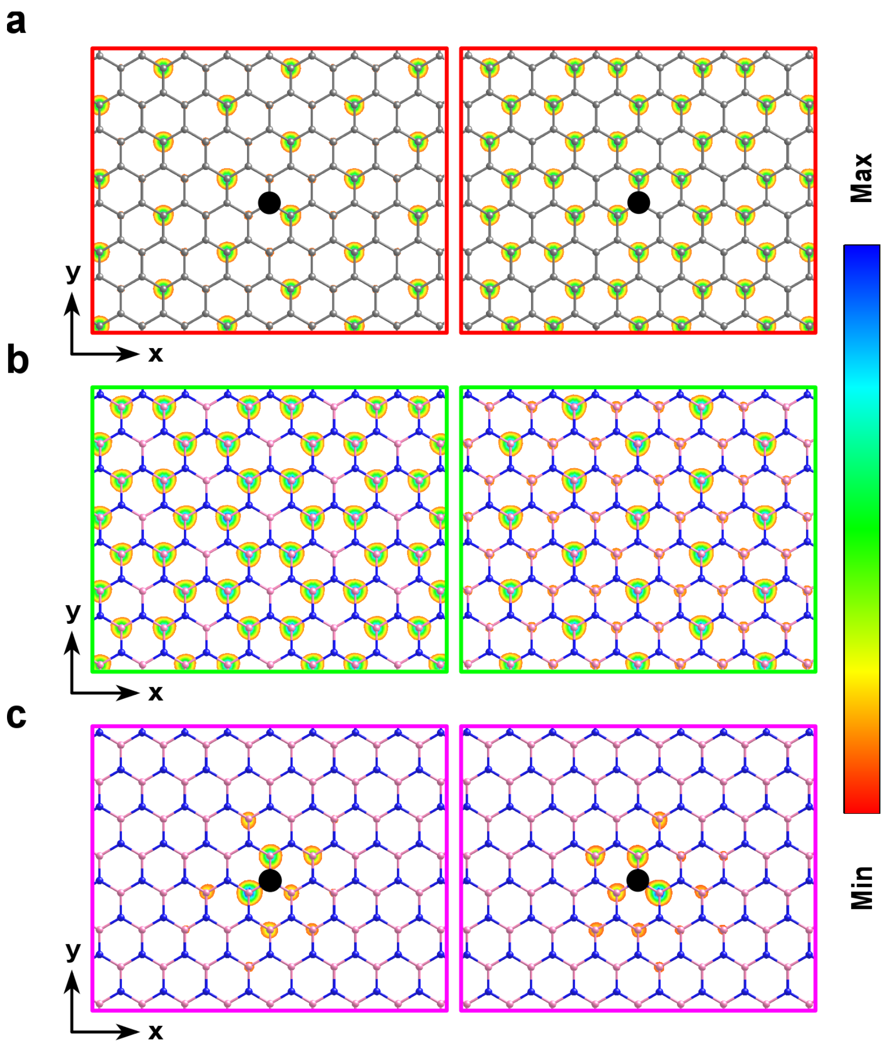


Figure S4: Two-dimensional projections of the probability density associated to the electron component of the electron-hole pairs of double-degenerate excitations with (a) graphene delocalized character, (b) h-BN delocalized and (c) localized character. The corresponding position of the hole is marked by a black dot.

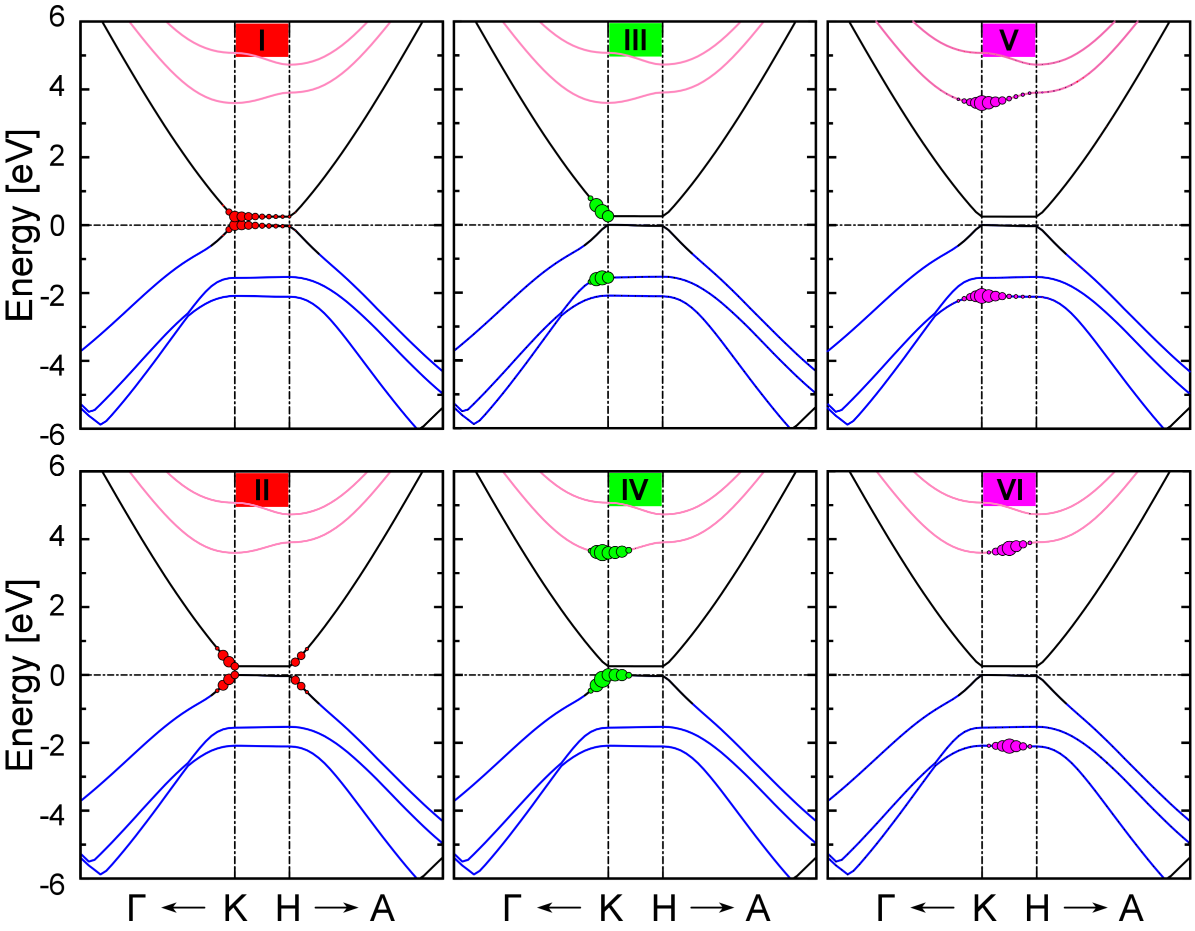


Figure S5: Band contributions to the main excitations in the spectra of the B-g-B heterostructure, given by the corresponding weights (Eq. 1). The size of the colored circles are quantitatively representative of the weight of the corresponding quasi-particle states. The band character is indicated by the color code of the atomic species (C: grey, N: blue, B: pink).

according to the notation introduced in the main text. For both heterostructures, the first excitations (I and II) are graphene interband transitions occurring along the K-H path (I) or in its vicinity (II). Excitations III and IV have charge-transfer character with the electron and the hole being situated on either graphene or h-BN layer. Specifically, excitation III stems from the N-like VBM-1 targeting the lowest unoccupied graphene band, regardless of the position of the hole above or below graphene. Excitation IV is characterized by transitions from the highest occupied graphene band to the B-like CBM+1. Excitons V and VI stem purely from the h-BN bands, within the K-H path.

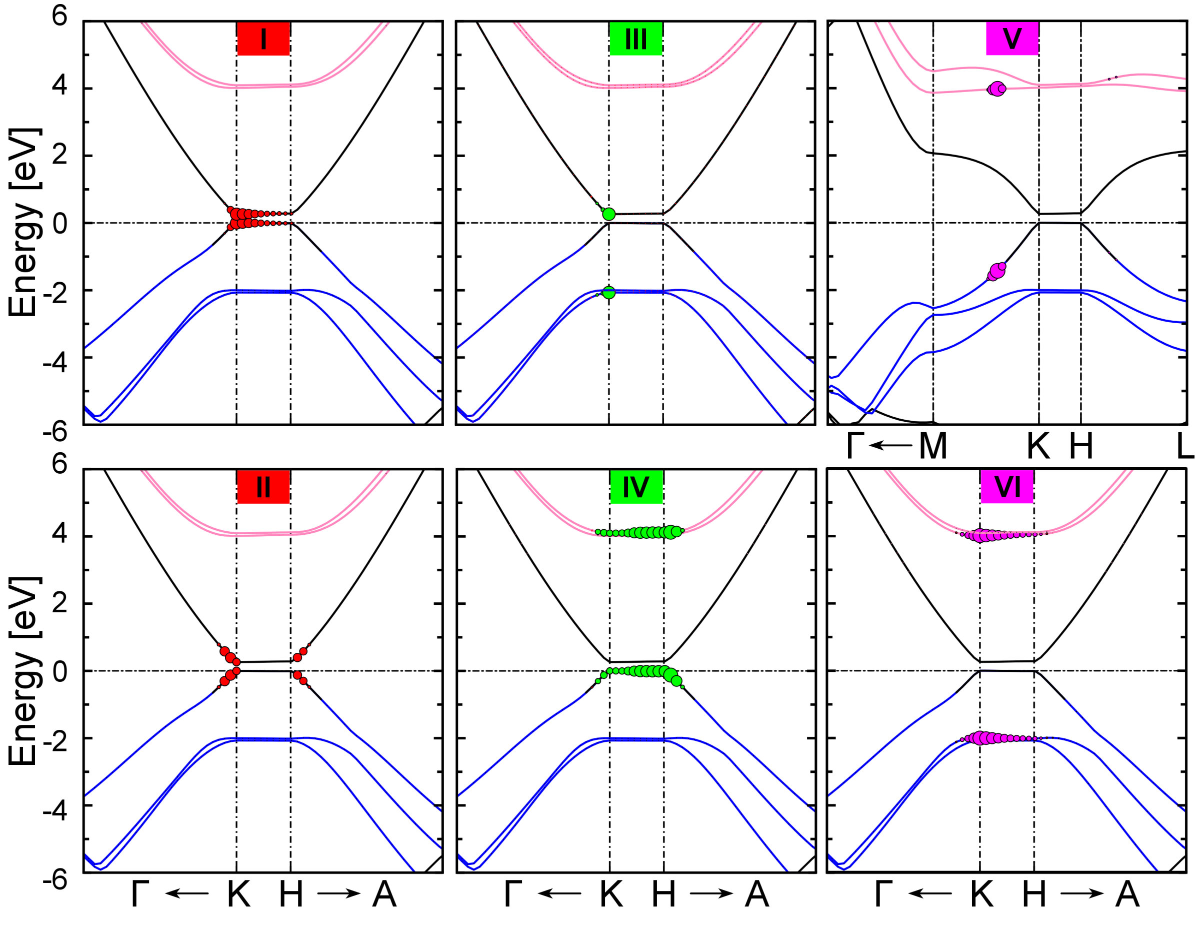


Figure S6: Band contributions to the main excitations in the spectra of B-g-C heterostructure, given by the corresponding weights (Eq. 1). The size of the colored circles are quantitatively representative of the weight of the corresponding quasi-particle states. The band character is indicated by the color code of the atomic species (C: grey, N: blue, B: pink).

In Fig. S6 we show the corresponding plots referred to the B-g-C heterostructure. No

significant differences appear regarding the interband transitions in graphene (excitations I and II). Conversely, the effects of the different stacking arrangements on the electronic wave-functions in the h-BN layers are reflected in the optical excitations where these states are involved. The interlayer excitations III and IV are again given by transition from h-BN to graphene bands (III) and from graphene to h-BN levels (IV). However, in this case, the distribution in **k**-space is slightly modified, as a consequence of the character of the h-BN bands, VBM-2/VBM-1 and CBM+1/CBM+2, along the K-H path (see also Fig. S2b). Even more pronounced differences appear in the h-BN excitons V and VI. Especially the former comes primarily from a region in the BZ between the high-symmetry points K and M.

## References

(1) Wirtz, L.; Marini, A.; Grüning, M.; Attaccalite, C.; Kresse, G.; Rubio, A. *Phys. Rev. Lett.* **2008**, *100*, 189701.
